# Supplementary material for: On the Complexity of Sequential Incentive Design
Source: arXiv:2007.08548 source file (2020-07-16)
Supplement: Supplementary file 1 [file Appendix_B.tex]

\section{}\label{example_appendix}
In this appendix, we illustrate with an example that the optimal value of the non-adaptive single-action behavior manipulation problem (NS-BMP), in which the principal is restricted to use only stationary deterministic incentive sequences, can be arbitrarily larger than the optimal value of the N-BMP. 

Consider the MDP given in Fig. \ref{fig:no_free_lunch_2}. The agent starts from the initial state $s_1$, and the target set is given by $B$$=$$\{s_4\}$. Suppose also that there are only two possible agent types, i.e., $\Theta$$=$$\{\theta_1,\theta_2\}$.

Consider the following \textit{stationary} incentive sequence which incentivizes two different actions from the initial state $s_1$:
\begin{align*}
    &\gamma(s_1,a_2)=1+\epsilon,\ \gamma(s_1,a_3)=1+\epsilon, \\ 
    &\gamma(s_2,a_2)=1+\epsilon, \ \gamma(s_3,a_2)=1+\epsilon.
\end{align*}
Under the provided incentive sequences, \textit{the} optimal stationary policy for the agent type $\theta_1$ satisfies $\pi(s_1)$$=$$a_2$ and $\pi(s_2)$$=$$a_2$. Therefore, under its optimal policy, the agent type $\theta_1$ first reaches the state $s_2$, and then the target state $s_4$ with probability 1. On the other hand, \textit{the} optimal stationary policy for the agent type $\theta_1$ satisfies $\pi(s_1)$$=$$a_3$ and $\pi(s_3)$$=$$a_2$. Unlike the type $\theta_1$, under its optimal policy, the agent type $\theta_2$ first reaches the state $s_3$, and then the target state $s_4$ with probability 1. Thus, the incentive sequence essentially reveals the true agent type. For the described incentive sequence, the worst-case total cost of behavior manipulation to the principal is $2$$+$$2\epsilon$. 

\begin{figure}[b!]
\begin{tikzpicture}[->, >=stealth', auto, semithick, node distance=2cm]

    \tikzstyle{every state}=[fill=white,draw=black,thick,text=black,scale=0.7]

    \node[state,initial below,initial text=] (s_1) {$s_1$};
    \node[state] (s_3) [ above right =10mm and 30 mm of s_1]  {$s_2$};
     \node[state] (s_4) [below right=10mm and 30 mm of s_1]  {$s_3$};
      \node[state] (s_5) [right=60mm of s_1]  {$s_4$};

\path
(s_1)  edge  [loop above=10]    node[]{\footnotesize{$a_1,(0,0)$}}     (s_1)
(s_3)  edge  [loop below=10]    node{\footnotesize{$a_1,(0,0)$}}     (s_3)
(s_4)  edge  [loop above=10]    node{\footnotesize{$a_1,(0,0)$}}     (s_4)

(s_1)	 edge     node[rotate=20, xshift= 0cm, yshift=-0cm,below ]{\footnotesize{$a_2,(-1,-2)$}}     (s_3)
(s_1)	 edge     node[rotate=-20,xshift= -0cm, yshift=-0cm,below]{\footnotesize{$a_3,(-2,-1)$}}     (s_4)

(s_3)	 edge     node[rotate=-20,xshift= -0.75cm ]{\footnotesize{$a_2,(-1,x)$}}     (s_5)
(s_4)	 edge     node[rotate=20, below]{\footnotesize{$a_2,(x,-1)$}}     (s_5)
(s_5)  edge  [loop right=20]    node{}     (s_5);
\end{tikzpicture}
\caption{An MDP example to illustrate that the optimal value of the NS-BMP may be arbitrarily larger than the optimal value of the N-BMP. Tuples $(a,(r_1,r_2))$ next to arrows consist of the action $a$, the reward $\mathcal{R}_{\theta_1}(s,a)$$=$$r_1$ for the type $\theta_1$, and the reward $\mathcal{R}_{\theta_2}(s,a)$$=$$r_2$ for the type $\theta_2$. The parameter $x$$<$$-1$.}
\label{fig:no_free_lunch_2}
\end{figure}

Now, let us consider \textit{deterministic stationary} incentive sequences. The principal can incentivize only a single action from the initial state $s_1$ under such incentive sequences. In order to ensure that the agent reaches the target state $s_4$ regardless of its true type $\theta^{\star}$, the principal must offer \textit{either} $\gamma(s_1,a_2)$$=$$2$$+$$\epsilon$ \textit{or} $\gamma(s_1,a_3)$$=$$2$$+$$\epsilon$. Therefore, unlike the incentive sequence described above, it is not possible for the principal to reveal the true agent type using deterministic stationary incentive sequences. As a result, it can be shown that the minimum total cost of behavior manipulation to the principal is $2$$-$$x$$+$$2\epsilon$. Hence, by choosing the parameter $x$ appropriately, we can make the minimum total cost to the principal arbitrarily larger than the minimum total cost of the stationary incentive sequences.
